# Supplementary material for: Specification-Guided Component-Based Synthesis from Effectful Libraries
Source: arXiv:2209.02752 source file (2022-09-06)
Supplement: Supplementary file 1 [file morpheusaddendum.pdf]

# Transforming Symbolic Transducers into Verifiable Parser Combinators*

## Subtitle†

Anonymous Author(s)

***Keywords:*** keywords

## 1 Supplemental Material for the Main Paper

### 1.1 The Language of expressions

Below we give the syntax for $L$-expressions, used in the main paper:

| | | |
|---|---|---|
| x, y, z, r, $v$ | | ∈ variables, c ∈ constants |
| | | first order functions and expressions |
| fun (f) | := | $\lambda$ x : t . e |
| value (v) | := | x \| C $\overline{x : \tau}$ \| c |
| exp (e) | := | value |
| | | \| f v \| let x = e in e \| fold f v v |
| | | \| match v with C $\overline{\text{e}}$ -> e else e |
| | | \| !r \| r := v \| ref v |

**Table 1.** Core syntax for $L$-expressions

### 1.2 Typing Semantics for expressions

Fig. 1 presents typing semantics for $L$-expressions. Each typing judgment is of the form $\Sigma \vdash \text{e} : \tau$, saying, in a typing environment $\Sigma$, an $L$ expression has a type $\tau$.

### 1.3 Evaluation Semantics for PST

Fig. 2 presents a full list of evaluation rules for our PST definition discussed in the Overview Section in the main paper.

### 1.4 Evaluation Semantics for CPSTs

Figure 3 presents a full list of evaluation rules for CPSTs.

### 1.5 Typing Semantics PST

Figure 4 presents full list of typing rules for a PST

### 1.6 Typing Semantics for CPST

Fig. 5 presents full list of typing rules for CPSTs and their combinators.

$$\text{T-fun}\ \frac{\Sigma, \text{x} : \tau \vdash e : \text{state}\ \{\phi\}\ t1\{\phi'\}}{\Sigma \vdash \lambda\ \text{x} : \text{t.e} : \text{state}\ \{\phi\}\ t1\{\phi'\}}$$

$$\text{T-app}\ \frac{\Sigma \vdash f : (\text{x} : t \to \text{state}\ \{\phi\}\ t1\{\phi'\} \qquad \Sigma \vdash \text{v1} : t}{\Sigma \text{f v} \vdash \text{state}\ \{\phi[\text{v1/x}]\}\ t1\{\phi'[\text{v1/x}]\}}$$

$$\text{T-match}\ \frac{\begin{array}{cc} \Sigma \vdash v : \tau & \Sigma \vdash C\overline{e} : \tau \\ \Sigma_{true} = \Sigma, v : \tau, v = C\overline{e} & \Sigma_{false} = \Sigma, v : \tau, v \neq C\overline{e} \\ \Sigma_{true} \vdash e1 : \tau_m & \Sigma_{false} \vdash e2 : \tau_m \end{array}}{\Sigma \vdash\ \text{match v with C}\overline{e} \to \text{e1 else e2} : \tau_m}$$

$$\text{T-let}\ \frac{\begin{array}{c} \Sigma \vdash e1 : \text{state}\ \{\phi 1\}\ t1\{\phi 1'\} \\ \Sigma, x : t1 \vdash e2 : \text{state}\ \{\phi 2\}\ t2\ \{\phi 2'\} \end{array}}{\Sigma \vdash \text{let x = e1 in e2} : \text{state}\ \{\text{bind}_{\text{pre}}\}\ t2\{\text{bind}_{\text{post}}\}}$$

$$\text{T-frame}\ \frac{\begin{array}{c} \Sigma \vdash \text{e1} : \text{state}\ \{\phi\}\ t1\ \{\phi'\} \\ \text{footprint}(\phi 1)\ \cap\ \text{footprint}(\phi_{\text{frame}}) = \{\} \end{array}}{\Sigma \vdash: \text{e1} : \text{state}\ \{\phi_{\text{frame}} \wedge \phi\}\ t1\ \{\phi_{\text{frame}} \wedge \phi'\}}$$

$$\text{T-ref}\ \frac{\Sigma \vdash \text{v} : t}{\Sigma \vdash: \text{refv} : ref t}$$

$$\text{T-deref}\ \frac{\Sigma \vdash \text{r} : ref t}{\Sigma \vdash: \text{!r} : t}$$

$$\text{T-assign}\ \frac{\Sigma \vdash \text{r} : ref t \qquad \Sigma \vdash v : t}{\Sigma \vdash: \text{r := v} : unit}$$

$$\text{T-fold}\ \frac{\begin{array}{c} \Sigma \vdash \text{f} : (x : t \to (\text{state}\{\phi\} y : tac\{\phi'\})) \\ \Sigma \vdash ac : tac \qquad \Sigma \vdash \text{l} : t \qquad \Sigma \vdash \text{Inv} \\ \Sigma \vdash \text{Inv}_{\text{pre}} \wedge \text{Inv}_{\text{ind}} \wedge \text{Inv}_{\text{post}} \end{array}}{\Sigma \vdash: \text{fold f ac l} : (\text{state}\{\text{Inv h}\} v : tac\{\text{Inv h}'\})}$$

**Figure 1.** Typing Semantics for $L$ expressions

*Title note
†Subtitle note

*PL'18, January 01–03, 2018, New York, NY, USA*
2021.

$$\boxed{(\mathcal{H}, q); c \Rightarrow (\mathcal{H}, q') \mid (\mathcal{H}, q); c \Rightarrow (\mathcal{H}, v)}$$

$$\text{S-P-}\mathcal{I}\ \frac{q_\bot \notin Q \qquad (\mathcal{H}; \mathcal{I}) \to (\mathcal{H}'; \_)}{(\mathcal{H}, q_\bot) \Rightarrow (\mathcal{H}, q_0)}$$

$$\text{S-P-Base}\ \frac{\begin{array}{c} \delta = (p \xrightarrow{\phi/\mathsf{f}} q) \\ [\![\phi]\!]\mathcal{H} = true \qquad (p \xrightarrow{\phi'/\mathsf{f}'} q') \in \mathsf{R}\backslash\delta \\ [\![\phi']\!]\mathcal{H} = false \\ (\mathcal{H}; \mathsf{f}) \Downarrow (\mathcal{H}'; \_) \end{array}}{(\mathcal{H}, p); \delta \Rightarrow (\mathcal{H}', q)}$$

$$\text{S-P-Ind}\ \frac{\begin{array}{cc} (\mathcal{H}, p); \mathsf{p_{k-1}}^{(p,q)} \Rightarrow (\mathcal{H}', q) & \delta = (q \xrightarrow{\phi/\mathsf{f}} r) \\ [\![\phi]\!]\mathcal{H}' = true & (q \xrightarrow{\phi'/\mathsf{f}'} r') \in \mathsf{R}\backslash\delta \\ [\![\phi']\!]\mathcal{H}' = false & (\mathcal{H}'; \mathsf{f}) \Downarrow (\mathcal{H}''; \_) \end{array}}{(\mathcal{H}, p); \mathsf{p_k}^{(p,r)} \Rightarrow (\mathcal{H}'', r)}$$

$$\text{S-P-Err}\ \frac{\begin{array}{c} \delta = (p \xrightarrow{\phi/\mathsf{f}} err) \qquad (p \xrightarrow{\phi'/\mathsf{f}'} q') \in R \setminus \delta \\ [\![\phi]\!]\mathcal{H} = true \qquad (p \xrightarrow{\phi'/\mathsf{f}'} q')\ [\![\phi']\!]\mathcal{H} = false \\ (\mathcal{H}; \mathsf{f}) \Downarrow (\mathcal{H}'; Err) \end{array}}{(\mathcal{H}, p); \delta \Rightarrow (\mathcal{H}', Err)}$$

$$\text{S-P-Act}\ \frac{\begin{array}{c} \delta = (p \xrightarrow{\phi/\mathsf{f}} q) \qquad (q \in F) \qquad \mathcal{A}(q) = \mathsf{e_q} \\ (p \xrightarrow{\phi'/\mathsf{f}'} q') \in R \setminus \delta \\ [\![\phi]\!]\mathcal{H} \qquad (p \xrightarrow{\phi'/\mathsf{f}'} q')\ [\![\phi']\!]\mathcal{H} = false \\ (\mathcal{H}; \mathsf{f}) \Downarrow (\mathcal{H}'; \_) \qquad (\mathcal{H}'; \mathsf{e_q}) \Downarrow (\mathcal{H}''; v) \end{array}}{(\mathcal{H}, p); \delta \Rightarrow (\mathcal{H}'', \mathsf{Val\ v})}$$

$$\text{S-P-L}\ \frac{\begin{array}{c} paths(PST) = \{\mathsf{p_{k1}}^{(q_0, q_{f1 \in F})}, \mathsf{p_{k2}}^{(q_0, q_{f2 \in F})}\} \\ (\mathcal{H}, q_0); \mathsf{p_{k1}}^{(q_0, q_{f \in F})} \Rightarrow (\mathcal{H}', \mathsf{vleft}) \end{array}}{(\mathcal{H}, q_0); PST \Rightarrow (\mathcal{H}', \mathsf{vleft})}$$

$$\text{S-P-R}\ \frac{\begin{array}{c} paths(PST) = \{\mathsf{p_{k1}}^{(q_0, q_{f1 \in F})}, \mathsf{p_{k2}}^{(q_0, q_{f2 \in F})}\} \\ (\mathcal{H}, q_0); \mathsf{p_{k2}}^{(q_0, q_{f2 \in F})} \Rightarrow (\mathcal{H}'', \mathsf{vright}) \end{array}}{(\mathcal{H}, q_0); PST \Rightarrow (\mathcal{H}'', \mathsf{vright})}$$

$$\text{S-P-Loop}\ \frac{\begin{array}{c} \delta = (p \xrightarrow{\phi/\mathsf{f}} q) \\ [\![\phi]\!]\mathcal{H} = true \qquad (p \xrightarrow{\phi'/\mathsf{f}'} q') \in \mathsf{R}\backslash\delta \\ [\![\phi']\!]\mathcal{H} = false \\ (\mathcal{H}; \mathsf{f}) \Downarrow (\mathcal{H}'; \_) \end{array}}{(\mathcal{H}, p); \delta \Rightarrow (\mathcal{H}', p)}$$

**Figure 2.** Evaluation rules for PST

$$\boxed{(\mathcal{H}, \mathsf{T}) \Rrightarrow (\mathcal{H}', v) \mid (\mathcal{H}, \mathsf{T}) \Rrightarrow (\mathcal{H}', T')}$$

$$\text{CS-}\iota\ \frac{(\mathcal{H}; q_\bot) \Rightarrow^* (\mathcal{H}'; v)}{(\mathcal{H}, \iota\mathsf{T}_0) \Rrightarrow (\mathcal{H}', v)}$$

$$\text{CS-bind}\ \frac{\begin{array}{c} (\mathcal{H}, \mathsf{T}_1) \Rrightarrow (\mathcal{H}', v1) \qquad v1 = Valv \\ \{\lambda x : t.\mathsf{T}_2\}_{\mathsf{x=v}} \Rrightarrow_\alpha [\,\mathsf{x} \mapsto \mathsf{v}]\ \mathsf{T}_2 \\ (\mathcal{H}', [\,\mathsf{x} \mapsto \mathsf{v}]\ \mathsf{T}_2) \Rrightarrow (\mathcal{H}'', v2) \end{array}}{(\mathcal{H}, (\mathsf{T}_1 \gg\!= (\lambda x : t.\mathsf{T}_2))) \Rrightarrow (\mathcal{H}'', v2)}$$

$$\text{CS-seq}\ \frac{\begin{array}{c} (\mathcal{H}, \mathsf{T}_1) \Rrightarrow (\mathcal{H}', v1) \qquad v1 = Valv \\ (\mathcal{H}'[\,inp := v\,], \mathsf{T}_2) \Rrightarrow (\mathcal{H}'', v2) \end{array}}{(\mathcal{H}, (\mathsf{T}_1 \mathsf{o} \mathsf{T}_2)) \Rrightarrow (\mathcal{H}'', v2)}$$

$$\text{CS-L}\ \frac{(\mathcal{H}, \mathsf{T}_1) \Rrightarrow (\mathcal{H}', v1)}{(\mathcal{H}, (\mathsf{T}_1 \mid \mathsf{T}_2)) \Rrightarrow (\mathcal{H}', \mathsf{Inl}\ (v1))}$$

$$\text{CS-R}\ \frac{(\mathcal{H}, \mathsf{T}_2) \Rrightarrow (\mathcal{H}'', v2)}{(\mathcal{H}, (\mathsf{T}_1 \mid \mathsf{T}_2)) \Rrightarrow (\mathcal{H}'', \mathsf{Inr}\ (v2))}$$

$$\text{CS-loop}\ \frac{\begin{array}{c} (\mathcal{H}, \mathsf{T}) \Rrightarrow (\mathcal{H}', v) \qquad \mathsf{v = Val\ y} \\ (\mathcal{H}'; (f\ y\ b)) \Downarrow (\mathcal{H}''; b') \end{array}}{(\mathcal{H}, (\mathsf{foldT\ T\ f\ b})) \Rrightarrow (\mathcal{H}'', (\mathsf{foldT\ T\ f\ b'}))}$$

$$\text{CS-break}\ \frac{(\mathcal{H}, \mathsf{T}) \Rrightarrow (\mathcal{H}', v) \qquad \mathsf{v = Err}}{(\mathcal{H}, (\mathsf{foldT\ T\ f\ b})) \Rrightarrow (\mathcal{H}', b)}$$

**Figure 3.** Evaluation rules for CPSTs, $\Rrightarrow^*$ represents multi-step evaluation for a PST

**Paths Typing** $\boxed{\Gamma \vdash \mathsf{p_k}^{(p,q)} : \tau}$

$$\text{T-P-Base}\ \frac{\delta = (p, \phi_g, \mathsf{f}, q) \quad q \neq err \quad \Sigma(\mathsf{f}) = ((\mathsf{i} : \mathsf{t}) \to \tau) \quad \tau = \mathsf{eff}\ \{\phi\}\mathsf{t}\{\phi'\} \quad \Gamma_{\mathsf{ext}} = \Gamma, i, (\phi_g\ \mathsf{i}\ \mathsf{h})}{\Gamma_{\mathsf{ext}} \vdash \delta : \mathsf{eff}\ \{\phi\}\mathsf{t}\{\phi'\}}$$

$$\text{T-P-Ind}\ \frac{\Gamma_1 \vdash \mathsf{p_{k-1}}^{(p,q)} : (\mathsf{eff}\ \{\phi_1\}\ \mathsf{t1}\ \{\phi_{1'}\}) \quad \mathsf{term}(\mathsf{p_{k-1}}) = \mathsf{start}(\mathsf{p_1}) \quad \Gamma_2 \vdash \mathsf{p_1}^{(q,r)} : (\mathsf{eff}\ \{\phi_2\}\ \mathsf{t2}\ \{\phi_{2'}\}) \quad \Gamma = \Gamma_1 @ \Gamma_2}{\Gamma \vdash \mathsf{p_k}^{(p,r)} : \mathsf{eff}\ \{\mathsf{path_{pre}}\}\ \mathsf{t2}\ \{\mathsf{path_{post}}\}}$$

$$\text{T-P-Error}\ \frac{\delta = (p, \phi_g, \mathsf{f}, \mathsf{err}) \quad \Sigma(\mathsf{f}) = ((\mathsf{i} : \mathsf{t}) \to \tau) \quad \tau = \mathsf{eff}\ \{\phi\}\ \mathsf{t}\ \{\phi'\} \quad \Gamma_{\mathsf{ext}} = \Gamma, i, (\phi_g\ \mathsf{i}\ \mathsf{h}) \quad \mathsf{eff'} = \mathsf{eff} \sqcup \mathsf{exc} \quad \phi'^{*} = \forall\ \mathsf{h}\ \mathsf{v}\ \mathsf{h'}.(\mathsf{v} = \mathsf{Err}) \wedge \phi'}{\Gamma_{\mathsf{ext}} \vdash \mathsf{p_1}^{(p,\mathsf{err})} : \mathsf{eff'}\ \{\phi\}\ \mathsf{result}\ \mathsf{t}\ \{\phi'^{*}\}}$$

$$\text{T-P-Act}\ \frac{\delta = (p, \phi_g, \mathsf{f}, \mathsf{q}) \quad (\mathsf{q} \in F \setminus \mathsf{err}) \quad \Sigma(\mathsf{f}) = ((\mathsf{i} : \mathsf{t}) \to \tau) \quad \tau = \mathsf{eff}\ \{\phi\}\ \mathsf{t}\ \{\phi'\} \quad \Gamma_{\mathsf{ext}} = \Gamma, i, (\phi_g\ \mathsf{i}\ \mathsf{h}) \quad \mathcal{A}(\mathsf{q}) = \mathsf{e_q} \quad \Sigma(\mathsf{e_q}) = \mathsf{eff}\ \{\phi1\}\ \mathsf{t1}\ \{\phi1'\}}{\Gamma_{\mathsf{ext}} \vdash \mathsf{p_1}^{(p,\mathsf{q}\in F)} : \mathsf{eff}\ \{\mathsf{act_{pre}}\}\ \mathsf{t1}\ \{\mathsf{act_{post}}\}}$$

$$\text{T-P-Loop}\ \frac{\delta = (p, \phi_g, \mathsf{f}, p) \quad \Sigma(\mathsf{f}) = ((\mathsf{i} : \mathsf{t}) \to \tau) \quad \tau = \mathsf{eff}\ \{\phi\}\ \mathsf{t}\ \{\phi'\} \quad \Gamma_{\mathsf{ext}} = \Gamma, i, (\phi_g\ \mathsf{i}\ \mathsf{h}) \quad \Gamma_{\mathsf{ext}} \vdash \mathsf{Inv} \quad \Gamma_{\mathsf{ext}} \vdash \mathsf{Inv_{pre}} \wedge \mathsf{Inv_{ind}} \wedge \mathsf{Inv_{break}}}{\Gamma_{\mathsf{ext}} \vdash \mathsf{p_1}^{(p,p)} : \mathsf{eff}\ \{\mathsf{Inv}\ \mathsf{h}\}\ \mathsf{t}\ \{\mathsf{Inv}\ \mathsf{h'}\}}$$

**PST Path Summation** $\boxed{\Gamma \vdash \mathsf{PST} : \tau}$

$$\text{T-P-Sum}\ \frac{paths(PST) = \{\mathsf{p_{k1}}^{(q0,(q\in F))}, \mathsf{p_{k1}}^{(q0,(r\in F))}\} \quad \Gamma_1 \vdash \mathsf{p_{k1}}^{(q0,(q\in F))} : \mathsf{eff}\ \{\phi1\}\ \mathsf{t}\{\phi1'\} \quad \Gamma_2 \vdash \mathsf{p_{k2}}^{(q0,(r\in F))} : \mathsf{eff}\ \{\phi2\}\ \mathsf{t}\{\phi2'\}}{\Gamma_1 @ \Gamma_2 \vdash PST : \mathsf{eff}\{(\phi1 \wedge \phi2)\}\ \mathsf{t}\ \{(\phi1' \vee \phi2')\}}$$

**PST Subtyping** $\boxed{\Gamma \vdash \tau_1 <: \tau_2}$

$$\text{T-P-Sub}\ \frac{\Gamma \vdash (\phi_{\mathsf{ann}} \Rightarrow \phi_1) \quad \Gamma \vdash t1 <: \mathsf{t_{ann}} \quad \Gamma \vdash \mathsf{eff} <: \mathsf{eff_{ann}} \quad \Gamma \vdash (\phi_{1'} \Rightarrow \phi_{\mathsf{ann'}})}{\Gamma \vdash \mathsf{eff}\ \{\phi_1\}\ \mathsf{t1}\ \{\phi_{1'}\} <: \mathsf{eff_{ann}}\ \{\phi_{\mathsf{ann}}\}\ \mathsf{t_{ann}}\ \{\phi_{\mathsf{ann'}}\}}$$

**Figure 4.** Typing rules over PST paths

**CPST Typing** $\boxed{\Gamma \vdash \mathsf{T} : \tau}$

$$\text{T-Bind}\ \frac{\Gamma \vdash T1 : \mathsf{eff}\ \{\phi1\}\ t1\{\phi1'\} \quad \Gamma, x : t1 \vdash T2 : \mathsf{eff}\ \{\phi2\}\ t2\ \{\phi2'\}}{\Gamma \vdash T1 \gg= \lambda x.T2 : \mathsf{eff}\{\mathsf{CBind_{pre}}\}\ \mathsf{t2}\ \{\mathsf{CBind_{post}}\}}$$

$$\text{T-Alt}\ \frac{\Gamma \vdash T1 : \mathsf{eff}\ \{\phi1\}\ t\{\phi1'\} \quad \Gamma \vdash T2 : \mathsf{eff}\ \{\phi2\}\ t\ \{\phi2'\} \quad \mathsf{eff'} = \mathsf{eff} \sqcup \mathsf{nondet}}{\Gamma \vdash (T1 <|> T2) : \mathsf{eff}\{(\phi1 \wedge \phi2)\}\ t\ \{(\phi1' \vee (\phi2')\}}$$

$$\text{T-Fold}\ \frac{\begin{array}{c}\Gamma \vdash T : \mathsf{eff}\ \{\phi\}\ t\ \{\phi'\} \\ \Sigma(acc) = b \quad \Sigma(\mathsf{f} : (x : t, y : b) \to \mathsf{eff}\ \{\phi_f\}\ b\ \{\phi'_f\}) \\ pre = \forall \mathrm{h}, h_i, \mathrm{x}, \mathrm{y}(\phi\ h\ y) \wedge (\phi'(h\ x\ h_i) \Rightarrow \phi_f(h_i\ x\ y) \\ post = \forall \mathrm{h}, h_i, \mathrm{x}, \mathrm{y}, \mathrm{h'}\ \mathrm{y'}.(\phi'(h\ x\ h_i) \wedge \phi'_f(h_i\ y'\ h'\ x\ y) \\ \Gamma_{\mathsf{ext}} \vdash (\mathsf{T} \gg= \lambda\ \mathsf{x}.\mathsf{T_f}) : \mathsf{eff}\ \{pre\}\ b\ \{post\} \\ \Gamma_{\mathsf{ext}} \vdash \mathsf{Inv_{pre}} \wedge \mathsf{Inv_{ind}} \wedge \mathsf{Inv_{break}}\end{array}}{\Gamma \vdash (\mathsf{foldT\_}) : \mathsf{eff}\ \{\mathsf{Inv}\}\ \mathsf{b}\ \{\mathsf{Inv}\}}$$

**Figure 5.** Typing Transducer Compositions

## 2 Details of Soundness Theorems and Proofs

We prove the soundness of typing rules for *L*-expressions and CPSTs using traditional *preservation* and *progress* theorems, assuming *Heap Soundness*. While, the soundness of typing a PST is built inductively over paths typing and ⇒. We also extend the typing judgements to a configuration ($\mathcal{H}$;c) or ($\mathcal{H}$;v). A heap $\mathcal{H}$ in our evaluation rule is a list of references r1, r2,... to values v. To relate it to the logical heaps we use in our specification language h, h', etc. we define the following interpretation function:

$$\|.\| = empty$$

$$\|\mathcal{H}, (\mathsf{r} \mapsto_\tau \mathsf{v})\| = \mathsf{update}\|\mathcal{H}\|\ \mathsf{r}\ \mathsf{v}$$

**Definition 2.1** (Heap Soundness)**.** For all r and h, If $\Gamma \vdash$ (dom h r) ∧ (sel h r v) then $(\mathsf{r} \mapsto_\tau \mathsf{v}) \in \mathcal{H}$ for some value v.

Using this definition of interpretation function for a runtime $\mathcal{H}$ to an abstract heap h in our typing rules, we defined the notion of semantic entailment (⊨) in an environment Γ.

**Definition 2.2** (Semantic entailment)**.** $\Gamma \models \phi\ (\mathcal{H})$ iff $\Gamma \vdash \|\mathcal{H}\|$.

**Theorem 2.3** (Preservation)**.** *The preservation lemma for an L-expression* e *and a CPST* T*.*

1. *If* ($\mathcal{H}$ ;e) ⇓ ($\mathcal{H}'$; e') *and* Γ ⊢ ($\mathcal{H}$; e) : τ*, then* Γ ⊢ ($\mathcal{H}'$; e') : τ
2. *If* ($\mathcal{H}$; T) ⇛ ($\mathcal{H}'$; T') *and* Γ ⊢ ($\mathcal{H}$; T) : τ*, then* Γ ⊢ ($\mathcal{H}'$; T') : τ

*Proof.* Proof. The proof is based on inductive analysis on expression and CPST evaluations rules and and inversion of corresponding typing rules. □

**Theorem 2.4** (Progress)**.** *The progress theorem for an L-expression* e *and a CPST* T*, supposing that the specification logic has Heap Soundness.*

1. Γ ⊢ ($\mathcal{H}$;e) : τ*, then either* e *is a value or a function, or there exists a* e'*, such that* ($\mathcal{H}$; e) ⇓ ($\mathcal{H}'$; e')*.*
2. Γ ⊢ ($\mathcal{H}$; T) : τ*, then either, there exists a* PST $\mathsf{T}_{\mathsf{base}}$ *and* T *is of the form* $\mathsf{T}_{\mathsf{base}}$ *or there exists some CPST* T'*, such that* ($\mathcal{H}$; T) ⇛ ($\mathcal{H}'$; T')

*Proof.* The proof is based on case analysis for each evaluation rule in *L*-expression and CPST and using inversion of corresponding typing rules. □

**Lemma 2.5** (Soundness Path Typing)**.** *Given,* $\Gamma \vdash \mathsf{p_k}^{(p,q)}$ : eff $\{\phi_k\}$ $\mathsf{t_k}$ $\{\phi'_k\}$*. Also Given there exists some* $\mathcal{H}$*, such that* $\Gamma \models \phi_k(\mathcal{H})$*.*
*Then there exists* $\mathcal{H}'$*, such that:*

- *Either:* ($\mathcal{H}$, p);$\mathsf{p_k}^{(p,q)}$ ⇒ ($\mathcal{H}'$; v)*,* Γ ⊢ v : $\mathsf{t_k}$ *and* $\Gamma, \phi_k\ (\mathcal{H}) \models \phi'_k\ (\mathcal{H})\ \mathsf{v}\ (\mathcal{H}')$*.*
- *Or:* ($\mathcal{H}$, p);$\mathsf{p_k}^{(p,q)}$ ⇒ ($\mathcal{H}'$; q) *and* $\Gamma, \phi_k\ (\mathcal{H}) \models \phi'_k\ (\mathcal{H})\ (\mathcal{H}')$*.*

*Proof.* The proof is inductively defined on the length of the path, giving two cases:

1. **Base Case (k = 1)** : We do a case analysis on typing rule for path of length 1:
   - Case : T-P-Base: Inverting (T-P-Base) implies:

     a. ∃δ = (p, $\phi_\mathsf{g}$, f, q)
     b. Γ = $\Gamma_0$, $\phi_g$ i h , where h = $\|\mathcal{H}\|$
     c. Using the progress for Σ typing and
     d. Well-formed semantics of the Transducers.
     e. Using (a)-(d), The evaluation rule (S-P-Base) applies, thus:
     f. There exists a heap $\mathcal{H}'$ such that ($\mathcal{H}$, p); δ ⇒ ($\mathcal{H}'$; q).
     g. Using sound typing result (Theorem 2.4 and 2.3) for *L*-expression we get (Σ, $\phi \models \phi'\ \mathcal{H}\ \mathcal{H}'$.) Using (T-P-Base), The pre and post type annotations, $\phi_k = \phi$ and $\phi'_k = \phi'$. Given, Γ is parameterized over Σ, we have $\Gamma, \phi_k\ (\mathcal{H}) \models \phi'_k\ (\mathcal{H})\ (\mathcal{H}')$.
     h. f and g ⟹ soundness
   - Case : T-P-Error : Inverting (T-P-Error) implies:

     a. ∃δ = (p, $\phi_\mathsf{g}$, f, err),
     b. Γ = $\Gamma_0$, $\phi_g$ i h , where h = $\|\mathcal{H}\|$.
     c. Using the progress for Σ typing and
     d. Well-formed semantics of the Transducers.
     e. Using (a)-(d), The evaluation rule (S-P-Error) applies, thus:
     f. There exists a heap $\mathcal{H}'$ such that ($\mathcal{H}$, p); δ ⇒ ($\mathcal{H}'$; Err).
     g. Using sound typing result (Theorems 2.4 and 2.3) for *L*-expression we get (Σ, $\phi \models \phi'\ \mathcal{H}\ \mathcal{H}'$
     h. Using (T-P-Error), The pre and post type annotations, $\phi_k = \phi$ and $\phi'_k$ = ($\phi'$∧ v = Err). Given, Γ is parameterized over Σ, we have $\Gamma, \phi_k\ (\mathcal{H}) \models \phi'_k\ (\mathcal{H})\ (\mathcal{H}')$.
     i. Using (T-P-Error), $\mathsf{t_k}$ = result t and $\phi'_k$ = ($\phi'$∧ v = Err), thus v = Err : $\mathsf{t_k}$.
     j. f, h and i ⟹ soundness.
   - Case : T-P-Act Similar to above two cases, using (S-P-Act) and soundness over the action of the final state.
   - Case : T-P-Loop : This case uses the definition of the Inv and the Invariant checking predicates to prove

the soundness. Inverting (T-P-Loop) implies:

a. $\exists\delta = (\mathsf{p}, \phi_\mathsf{g}, \mathsf{f}, \mathsf{p})$
b. $\Gamma = \Gamma_0, \phi_g$ i h , where h = $||\mathcal{H}||$
c. Using the progress for $\Sigma$ typing and
d. Well-formed semantics of the Transducers.
e. Using (a)-(d), The evaluation rule (S-P-Loop) applies, thus:
f. There exists a heap $\mathcal{H}'$ such that $(\mathcal{H}, \mathsf{p}); \delta \Rightarrow (\mathcal{H}'; \mathsf{p})$.
g. Using sound typing result (Theorem 2.4 and 2.3) for $L$-expression we get ($\Sigma$, $\phi \models \phi'$ $\mathcal{H}$ $\mathcal{H}'$.) Using (T-P-Loop), The Invariant checking predicates contain all the cases, when the loop takes one no-iteration, 1-or-more iterations and when $\phi_g$ is false. Thus by construction of Invariant, $\Gamma_{ext} \models$ Inv $(\mathcal{H})$ $(\mathcal{H}')$.
h. f and g $\implies$ soundness

2. **Inductive Case (k > 1)** : The only typing rule applicable in this case:
   - T-P-Ind : Inverting the (T-P-Ind) rule implies:

a. $\exists$ a path of length (k-1), $(\mathsf{p_{k-1}}^{(p,q)})$, such that for some $\Gamma_1 \subseteq \Gamma \vdash (\mathsf{p_{k-1}}^{(p,q)})$ : eff $\{\phi_{k-1}\}$ $\mathsf{t_{k-1}}$ $\{\phi'_{k-1}\}$
b. $\exists$ a path of length (1), $(\mathsf{p_1}^{(q,r)})$, such that for some $\Gamma_2 \subseteq \Gamma \vdash (\mathsf{p_1}^{(q,r)})$ :eff $\{\phi_1\}$ $\mathsf{t_1}$ $\{\phi'_1\}$
c. terminal control state for $(\mathsf{p_{k-1}}^{(p,q)})$ = start control state $(\mathsf{p_1}^{(q,r)})$.
d. Using Induction Hypothesis on soundness of $(\mathsf{p_{k-1}}^{(p,q)})$ implies $(\mathcal{H}, \mathsf{p});(\mathsf{p_{k-1}}^{(p,q)}) \Rightarrow (\mathcal{H}_{int1}; \mathsf{q})$
e. $(\mathsf{p_1}^{(q,r)})$, implies $(\mathcal{H}_{int2}, \mathsf{p});(\mathsf{p_1}^{(q,r)}) \Rightarrow (\mathcal{H}'; \mathsf{r})$.
f. Using (T-P-Ind) $\Gamma \vdash \phi$ the guard for the $(\mathsf{p_1}^{(q,r)})$.
g. Main induction step : Using (T-P-Ind), $\mathsf{path_{pre}}$ implies $(\phi'_{k-1}$ $(\mathcal{H}_{int1})$ $\implies$ $(\phi_1$ $\mathcal{H}_{int2})$, thus, $(\mathcal{H}_{int2}; \mathsf{q}) \Rightarrow (\mathcal{H}'; \mathsf{r})$, thus (S-P-Ind) is applicable and $(\mathcal{H}, \mathsf{p});(\mathsf{p_k}^{(p,r)}) \Rightarrow (\mathcal{H}'; \mathsf{r})$.
h. Using Induction Hypothesis, $\Gamma_1, \phi_{k-1}$ $(\mathcal{H}) \models \phi'_{k-1}$ $(\mathcal{H})$ $(\mathcal{H}_{int1})$ and $\Gamma_2, \phi_1$ $(\mathcal{H}_{int2}) \models \phi'_1$ $(\mathcal{H}_{int2})$ $(\mathcal{H}')$ and Thus, $\Gamma_1 @ \Gamma_2 \vdash \mathsf{path_{pred}} \models \mathsf{path_{post}}$ $(\mathcal{H})$ $(\mathcal{H}_{int1})$ $(\mathcal{H}_{int2})$ $(\mathcal{H}')$, giving us our required proof of soundness for $\mathsf{p_k}^{(p,r)}$.
i. g and h $\implies$ soundness.

□

**Theorem 2.6** (Soundness PST). *Given a correctness specification $\tau$ = eff $\{\phi\}$ v: t $\{\phi'\}$ and a PST T, such that under some $\Gamma$, $\Gamma \vdash$ T : $\tau$, then if there there exists $\mathcal{H}$, such that $\Gamma \models \phi(\mathcal{H})$, then there exists a $\mathcal{H}'$, such that,*

- $(\mathcal{H}, q_0)$; T $\Rightarrow$ $(\mathcal{H}'; \mathsf{v})$
- $\Gamma \vdash$ v : t
- $\Gamma, \phi$ $(\mathcal{H}) \models \phi'$ $(\mathcal{H})$ v $(\mathcal{H}')$

*Proof.* The proof uses T-P-Sum rule, Inverting the rule implies:

1. $\exists$ two paths $\mathsf{p_{k1}}^{(q0,(q \in F))}$, and $\mathsf{p_{k1}}^{(q0,(r \in F))}$.
2. Using the soundness rule for paths (Lemma 2.5), either (S-P-L) or (S-P-R) apply.
3. Thus, $\exists$ either $\mathcal{H}'$, vleft or $\mathcal{H}''$, vright such that.
4. $(\mathcal{H}, q_0)$; PST $\Rightarrow$ $(\mathcal{H}'; \text{vleft})$. Or
5. $(\mathcal{H}, q_0)$; PST $\Rightarrow$ $(\mathcal{H}''; \text{vright})$.
6. Using (T-P-Sum) and Soundness of path typing (Lemma 2.5) $\Gamma \vdash$ vleft : t and vright : t, Thus, $\Gamma \vdash$ v : t.
7. Using (T-P-Sum) and Soundness of path typing (Lemma 2.5), $\Gamma, \phi1$ $(\mathcal{H}) \models \phi1'$ $(\mathcal{H})$ vleft $(\mathcal{H}')$ and $\Gamma, \phi2$ $(\mathcal{H}) \models \phi2'$ $(\mathcal{H})$ vright $(\mathcal{H}'')$.
8. Thus $\Gamma, \phi1 \wedge \phi2$ $(\mathcal{H}) \models (\phi1'$ $(\mathcal{H})$ vleft $(\mathcal{H}')) \vee (\phi1'$ $(\mathcal{H})$ vright $(\mathcal{H}''))$.
9. Using 4, 5, 6, 8 $\implies$ soundness condition.

□
