# Supplementary material for: Specification-Guided Component-Based Synthesis from Effectful Libraries
Source: arXiv:2209.02752 source file (2022-09-06)
Supplement: Supplementary file 3 [file supplement_pldi.tex]

%% For double-blind review submission, w/o CCS and ACM Reference (max submission space)
\documentclass[sigplan,10pt,review,anonymous]{acmart}
\settopmatter{printfolios=true,printccs=false,printacmref=false}
%% For double-blind review submission, w/ CCS and ACM Reference
%\documentclass[sigplan,review,anonymous]{acmart}\settopmatter{printfolios=true}
%% For single-blind review submission, w/o CCS and ACM Reference (max submission space)
%\documentclass[sigplan,review]{acmart}\settopmatter{printfolios=true,printccs=false,printacmref=false}
%% For single-blind review submission, w/ CCS and ACM Reference
%\documentclass[sigplan,review]{acmart}\settopmatter{printfolios=true}
%% For final camera-ready submission, w/ required CCS and ACM Reference
%\documentclass[sigplan]{acmart}\settopmatter{}

%% Conference information
%% Supplied to authors by publisher for camera-ready submission;
%% use defaults for review submission.
\acmConference[PL'18]{ACM SIGPLAN Conference on Programming Languages}{January 01--03, 2018}{New York, NY, USA}
\acmYear{2021}
\acmISBN{} % \acmISBN{978-x-xxxx-xxxx-x/YY/MM}
\acmDOI{} % \acmDOI{10.1145/nnnnnnn.nnnnnnn}
\startPage{1}

%% Copyright information
%% Supplied to authors (based on authors' rights management selection;
%% see authors.acm.org) by publisher for camera-ready submission;
%% use 'none' for review submission.
\setcopyright{none}
%\setcopyright{acmcopyright}
%\setcopyright{acmlicensed}
%\setcopyright{rightsretained}
%\copyrightyear{2018}           %% If different from \acmYear

%% Bibliography style
\bibliographystyle{ACM-Reference-Format}
%% Citation style
%\citestyle{acmauthoryear}  %% For author/year citations
%\citestyle{acmnumeric}     %% For numeric citations
%\setcitestyle{nosort}      %% With 'acmnumeric', to disable automatic
                            %% sorting of references within a single citation;
                            %% e.g., \cite{Smith99,Carpenter05,Baker12}
                            %% rendered as [14,5,2] rather than [2,5,14].
%\setcitesyle{nocompress}   %% With 'acmnumeric', to disable automatic
                            %% compression of sequential references within a
                            %% single citation;
                            %% e.g., \cite{Baker12,Baker14,Baker16}
                            %% rendered as [2,3,4] rather than [2-4].

%%%%%%%%%%%%%%%%%%%%%%%%%%%%%%%%%%%%%%%%%%%%%%%%%%%%%%%%%%%%%%%%%%%%%%
%% Note: Authors migrating a paper from traditional SIGPLAN
%% proceedings format to PACMPL format must update the
%% '\documentclass' and topmatter commands above; see
%% 'acmart-pacmpl-template.tex'.
%%%%%%%%%%%%%%%%%%%%%%%%%%%%%%%%%%%%%%%%%%%%%%%%%%%%%%%%%%%%%%%%%%%%%%

%% Some recommended packages.
\usepackage{wrapfig}
\usepackage{booktabs}   %% For formal tables:
                        %% http://ctan.org/pkg/booktabs
\usepackage{subcaption} %% For complex figures with subfigures/subcaptions
                        %% http://ctan.org/pkg/subcaption

\usepackage{listings} 
\lstset{columns=fullflexible,
        mathescape=true,
        comment=[l]{\%},
        literate=
               {<-}{$\leftarrow{}$}{1}
               {->}{$\rightarrow{}$}{1},
               morekeywords={state,stexc,nondet,Val,Err}
	    %morekeywords={fun,{,},if,then,else,return,state,stexc,nondet,Val,Err}
        }
\usepackage{semantic}
\usepackage{tikz,pgf}
\usepackage{stmaryrd}
\usepackage{xcolor}
\setpremisesspace{1cm}

\usepackage{authorcomments}

\usepackage{stmaryrd}

\definecolor{mygreen}{rgb}{0,0.6,0}
\definecolor{mygray}{rgb}{0.5,0.5,0.5}
\definecolor{mymauve}{rgb}{0.58,0,0.82}

\tikzoption{base font}{\def\tikz@base@textfont{#1}}
\tikzset{
  base font=\sffamily,
}
\usepackage{amsmath}
\usepackage{supertabular}
\usepackage{geometry}
\usepackage{ifthen}
\usepackage{alltt}%hack
\geometry{a4paper,dvips,twoside,left=22.5mm,right=22.5mm,top=20mm,bottom=30mm}
\usepackage{color}

\usepackage{multirow}
\usepackage{multicol}
\usepackage{semantic}
\usepackage{algpseudocode}
\usepackage[noend,noline]{algorithm2e}
\usepackage{pgfplots, pgfplotstable}
%\pgfplotsset{compat=1.7}
\pgfplotsset{compat=1.13}
\SetKwInput{KwData}{Input}
\SetKwInput{KwResult}{Output}

\begin{document}

%% Title information
\title[Effectful Component-Based Synthesis]
      {Specification-Guided Component-Based Synthesis from Effectful Libraries }         %% [Short Title] 
                                        %% when present, will be used in
                                        %% header instead of Full Title.
\titlenote{with title note}             %% \titlenote is optional;
                                        %% can be repeated if necessary;
                                        %% contents suppressed with 'anonymous'
\subtitle{Supplemental Material for the Main Paper}                     %% \subtitle is optional
\subtitlenote{with subtitle note}       %% \subtitlenote is optional;
                                        %% can be repeated if necessary;
                                        %% contents suppressed with 'anonymous'

%% Author information
%% Contents and number of authors suppressed with 'anonymous'.
%% Each author should be introduced by \author, followed by
%% \authornote (optional), \orcid (optional), \affiliation, and
%% \email.
%% An author may have multiple affiliations and/or emails; repeat the
%% appropriate command.
%% Many elements are not rendered, but should be provided for metadata
%% extraction tools.

%% Author with single affiliation.
\author{First1 Last1}
\authornote{with author1 note}          %% \authornote is optional;
                                        %% can be repeated if necessary
\orcid{nnnn-nnnn-nnnn-nnnn}             %% \orcid is optional
\affiliation{
  \position{Position1}
  \department{Department1}              %% \department is recommended
  \institution{Institution1}            %% \institution is required
  \streetaddress{Street1 Address1}
  \city{City1}
  \state{State1}
  \postcode{Post-Code1}
  \country{Country1}                    %% \country is recommended
}
\email{first1.last1@inst1.edu}          %% \email is recommended

%% Author with two affiliations and emails.
\author{First2 Last2}
\authornote{with author2 note}          %% \authornote is optional;
                                        %% can be repeated if necessary
\orcid{nnnn-nnnn-nnnn-nnnn}             %% \orcid is optional
\affiliation{
  \position{Position2a}
  \department{Department2a}             %% \department is recommended
  \institution{Institution2a}           %% \institution is required
  \streetaddress{Street2a Address2a}
  \city{City2a}
  \state{State2a}
  \postcode{Post-Code2a}
  \country{Country2a}                   %% \country is recommended
}
\email{first2.last2@inst2a.com}         %% \email is recommended
\affiliation{
  \position{Position2b}
  \department{Department2b}             %% \department is recommended
  \institution{Institution2b}           %% \institution is required
  \streetaddress{Street3b Address2b}
  \city{City2b}
  \state{State2b}
  \postcode{Post-Code2b}
  \country{Country2b}                   %% \country is recommended
}
\email{first2.last2@inst2b.org}         %% \email is recommended

%% Abstract
%% Note: \begin{abstract}...\end{abstract} environment must come
%% before \maketitle command
% \begin{abstract}
% \end{abstract}

%% 2012 ACM Computing Classification System (CSS) concepts
%% Generate at 'http://dl.acm.org/ccs/ccs.cfm'.
\begin{CCSXML}
<ccs2012>
<concept>
<concept_id>10011007.10011006.10011008</concept_id>
<concept_desc>Software and its engineering~General programming languages</concept_desc>
<concept_significance>500</concept_significance>
</concept>
<concept>
<concept_id>10003456.10003457.10003521.10003525</concept_id>
<concept_desc>Social and professional topics~History of programming languages</concept_desc>
<concept_significance>300</concept_significance>
</concept>
</ccs2012>
\end{CCSXML}

\ccsdesc[500]{Software and its engineering~General programming languages}
\ccsdesc[300]{Social and professional topics~History of programming languages}
%% End of generated code

%% Keywords
%% comma separated list
%%\keywords{Automatic Verification, Symbolic Transducers, Parser Combinators, Refinement Types, Effectful 
%%Verification.}  %% \keywords are mandatory in final camera-ready submission

%% \maketitle
%% Note: \maketitle command must come after title commands, author
%% commands, abstract environment, Computing Classification System
%% environment and commands, and keywords command.
\maketitle
\input{document}
%% Acknowledgments
\begin{acks}                            %% acks environment is optional
                                        %% contents suppressed with 'anonymous'
  %% Commands \grantsponsor{<sponsorID>}{<name>}{<url>} and
  %% \grantnum[<url>]{<sponsorID>}{<number>} should be used to
  %% acknowledge financial support and will be used by metadata
  %% extraction tools.
  This material is based upon work supported by the
  \grantsponsor{GS100000001}{National Science
    Foundation}{http://dx.doi.org/10.13039/100000001} under Grant
  No.~\grantnum{GS100000001}{nnnnnnn} and Grant
  No.~\grantnum{GS100000001}{mmmmmmm}.  Any opinions, findings, and
  conclusions or recommendations expressed in this material are those
  of the author and do not necessarily reflect the views of the
  National Science Foundation.
\end{acks}

%% Bibliography
\bibliography{paper}

%% %% Appendix
%% \appendix
%% \section{Appendix}

%% Text of appendix \ldots
%\input{supplimentary}
\end{document}
